# Supplementary material for: Formal Analysis of Lending Pools in Decentralized Finance
Source: arXiv:2206.01333 source file (2022-09-16)
Supplement: Supplementary file 1 [file appendices.tex]

\section{Additional figures}
\label{chapter:add-figures}

\SecSubSec{Modelling stock prices}

\begin{figure}[H]
  \centering
  \begin{subfigure}[H]{0.45\textwidth}
    \centering
    \includegraphics[width=\textwidth]{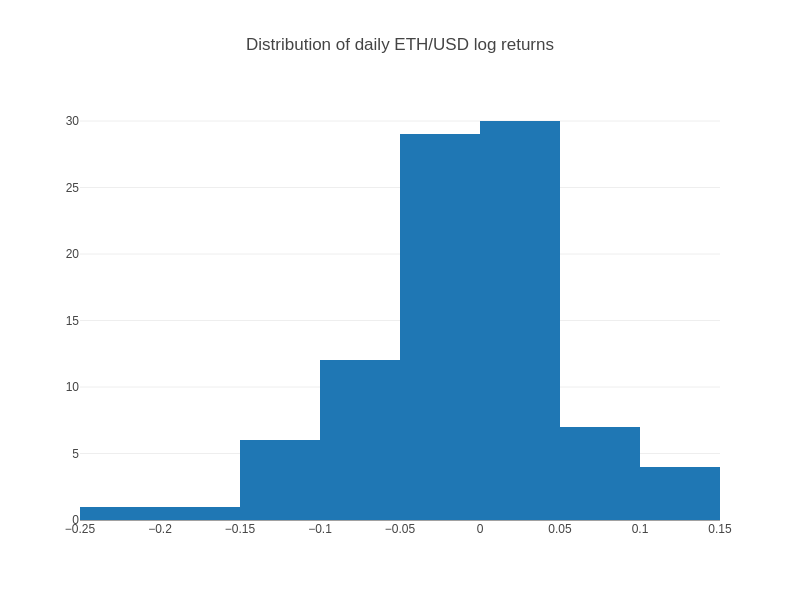}
    \caption{{\footnotesize 13/01/2018-14/04/2018}}
    \label{fig:eth-hist}
  \end{subfigure}
% \end{figure}
% \begin{figure} \ContinuedFloat
%   \centering
  \medskip
  \begin{subfigure}[H]{0.45\textwidth}
    \centering
    \includegraphics[width=\textwidth]{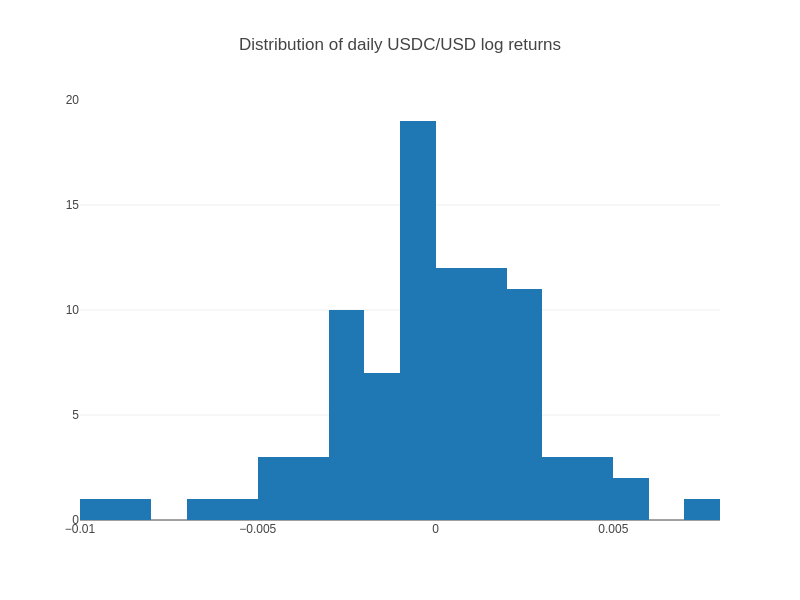}
    \caption{{\footnotesize 01/01/2020-01/04/2020}}
    \label{fig:usdc-hist}
  \end{subfigure}
  \medskip       
  \begin{subfigure}[H]{0.45\textwidth}
    \centering
    \includegraphics[width=\textwidth]{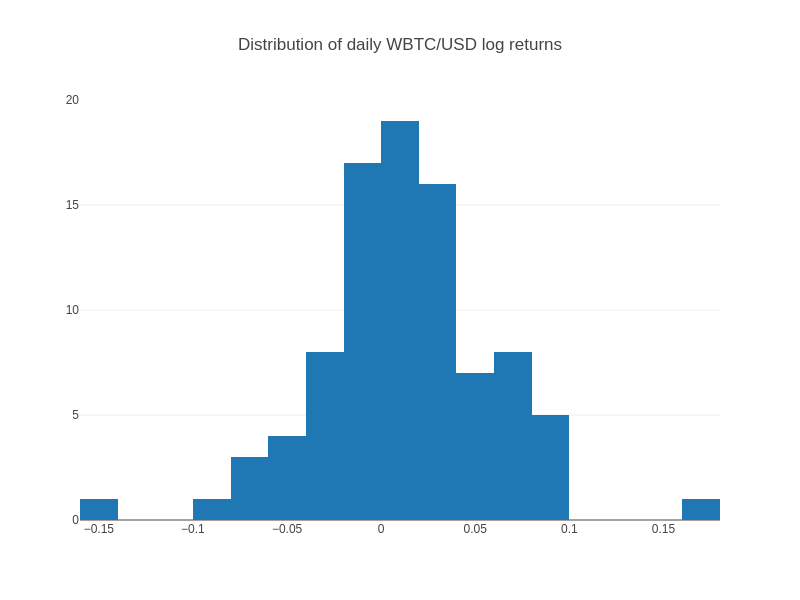}
    \caption{{\footnotesize 24/11/2020-23/02/2021}}
    \label{fig:wbtc-hist}
  \end{subfigure}
  \caption{Distributions of daily log returns computed from trimester closing prices}
  \label{fig:log-ret-hist}
\end{figure}

\begin{figure}[H]
  \centering
  \begin{subfigure}[H]{0.6\textwidth}
    \centering
    \includegraphics[width=\textwidth]{collateral-eth-wbtc.png}
    \caption{}    
    % \caption{Predictions based on GBM instantiated with ETH parameters, in prices model scenario eth-wbtc.}
    \label{fig:unnorm-coll-eth-wbtc}
  \end{subfigure}
  \medskip       
  \begin{subfigure}[H]{0.6\textwidth}
    \centering
    \includegraphics[width=\textwidth]{collateral-eth-usdc.png}
    \caption{}
    % \caption{Predictions based on GBM instantiated with ETH parameters, in prices model scenario eth-usdc.}
    \label{fig:unnorm-coll-eth-usdc}
  \end{subfigure}
  \medskip
  % \end{figure}
  % \begin{figure}[h] \ContinuedFloat
  %   \centering
  \begin{subfigure}[H]{0.6\textwidth}
    \centering
    \includegraphics[width=\textwidth]{collateral-usdc-wbtc.png}
    \caption{}    
    % \caption{Predictions based on GBM instantiated with USDC parameters, in prices model scenario usdc-wbtc.}         
    \label{fig:unnorm-coll-usdc-wbtc}
  \end{subfigure}
  \caption{Prices predictions for the collateral assets produced, for each scenario in \Cref{tab:prices-pairs}, by GBMs instantiated with the parameters in \Cref{tab:gbm-params}.}
  \label{fig:unnorm-coll-all}
\end{figure}

\begin{figure}[H]
  \centering
  \begin{subfigure}[H]{0.6\textwidth}
    \centering
    \includegraphics[width=\textwidth]{loan-eth-wbtc.png}
    \caption{}    
    % \caption{Predictions based on GBM instantiated with WBTC parameters, in prices model scenario eth-wbtc.}
    \label{fig:unnorm-loan-eth-wbtc}
  \end{subfigure}
  \medskip       
  \begin{subfigure}[H]{0.6\textwidth}
    \centering
    \includegraphics[width=\textwidth]{loan-eth-usdc.png}
    \caption{}    
    % \caption{Predictions based on GBM instantiated with USDC parameters, in prices model scenario eth-usdc.}
    \label{fig:unnorm-loan-eth-usdc}
  \end{subfigure}
  \medskip
  % \end{figure}
  % \begin{figure}[h] \ContinuedFloat
  %   \centering
  \begin{subfigure}[H]{0.6\textwidth}
    \centering
    \includegraphics[width=\textwidth]{loan-usdc-wbtc.png}
    \caption{}    
    % \caption{Predictions based on GBM instantiated with WBTC parameters, in prices model scenario usdc-wbtc.}         
    \label{fig:unnorm-loan-usdc-wbtc}
  \end{subfigure}
  \caption{Prices predictions for the loan assets produced, for each scenario in \Cref{tab:prices-pairs}, by GBMs instantiated with the parameters in \Cref{tab:gbm-params}.}
  \label{fig:unnorm-loan-all}
\end{figure}

\SecSubSec{Results of the statistical analysis}

\begin{figure}[H]
  \centering
  \includegraphics[scale=0.5,angle=90]{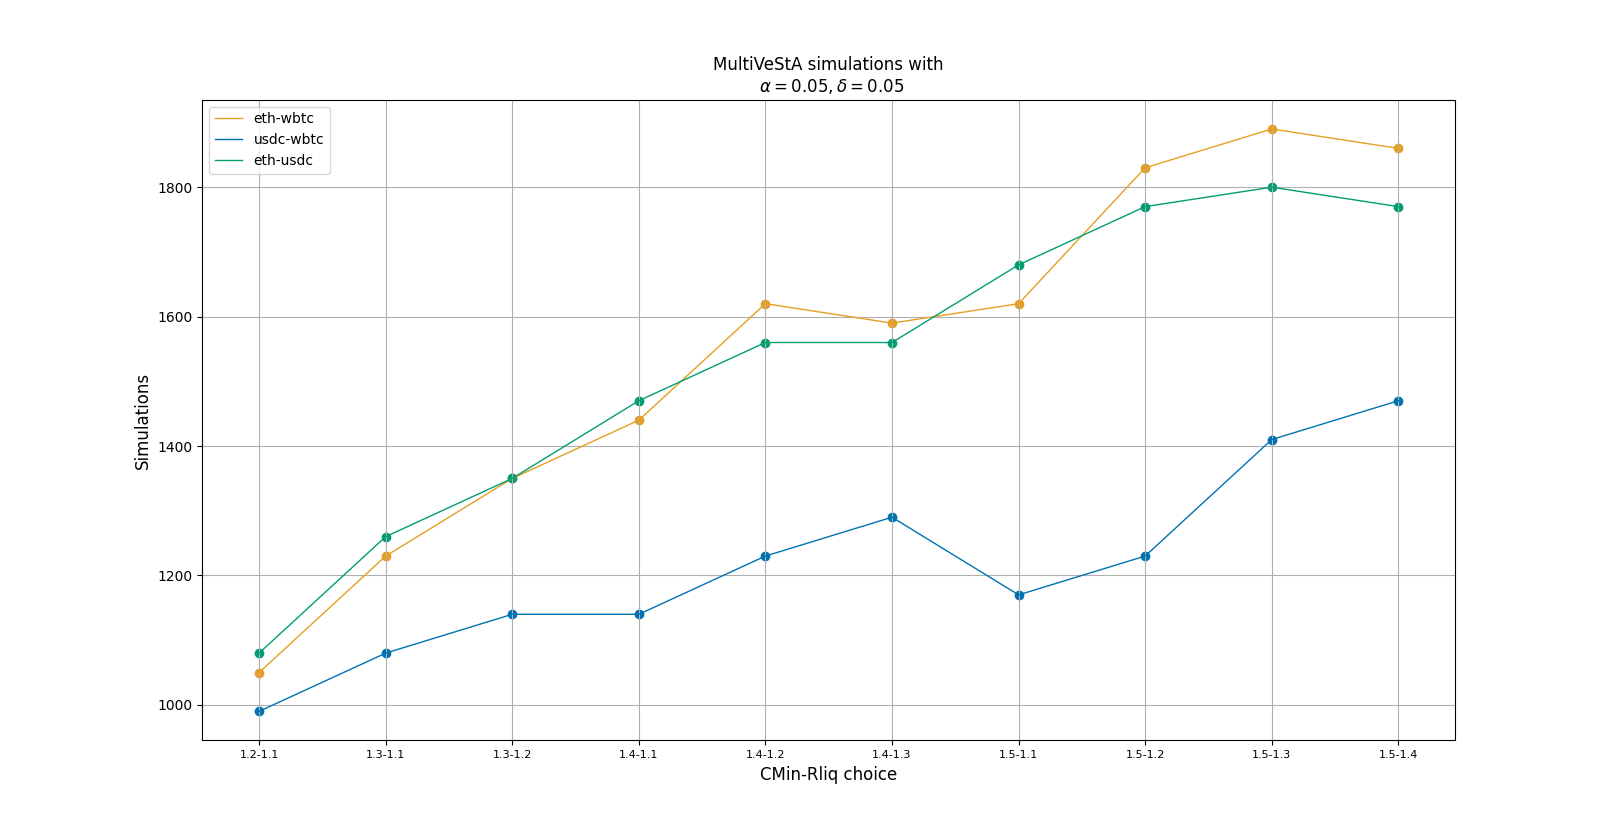}
  \caption{Number of LP simulations, per \texttt{CMin-rliq} choices, performed to obtain an acceptable approximation of the per-agent collateralization (\Cref{fig:3d-1-5,fig:3d-3-7,fig:3d-all}).}
  \label{fig:n-sims}
\end{figure}

\begin{figure}[H]
  \centering
  \begin{subfigure}[H]{\textwidth}
    \centering
    \includegraphics[angle=90]{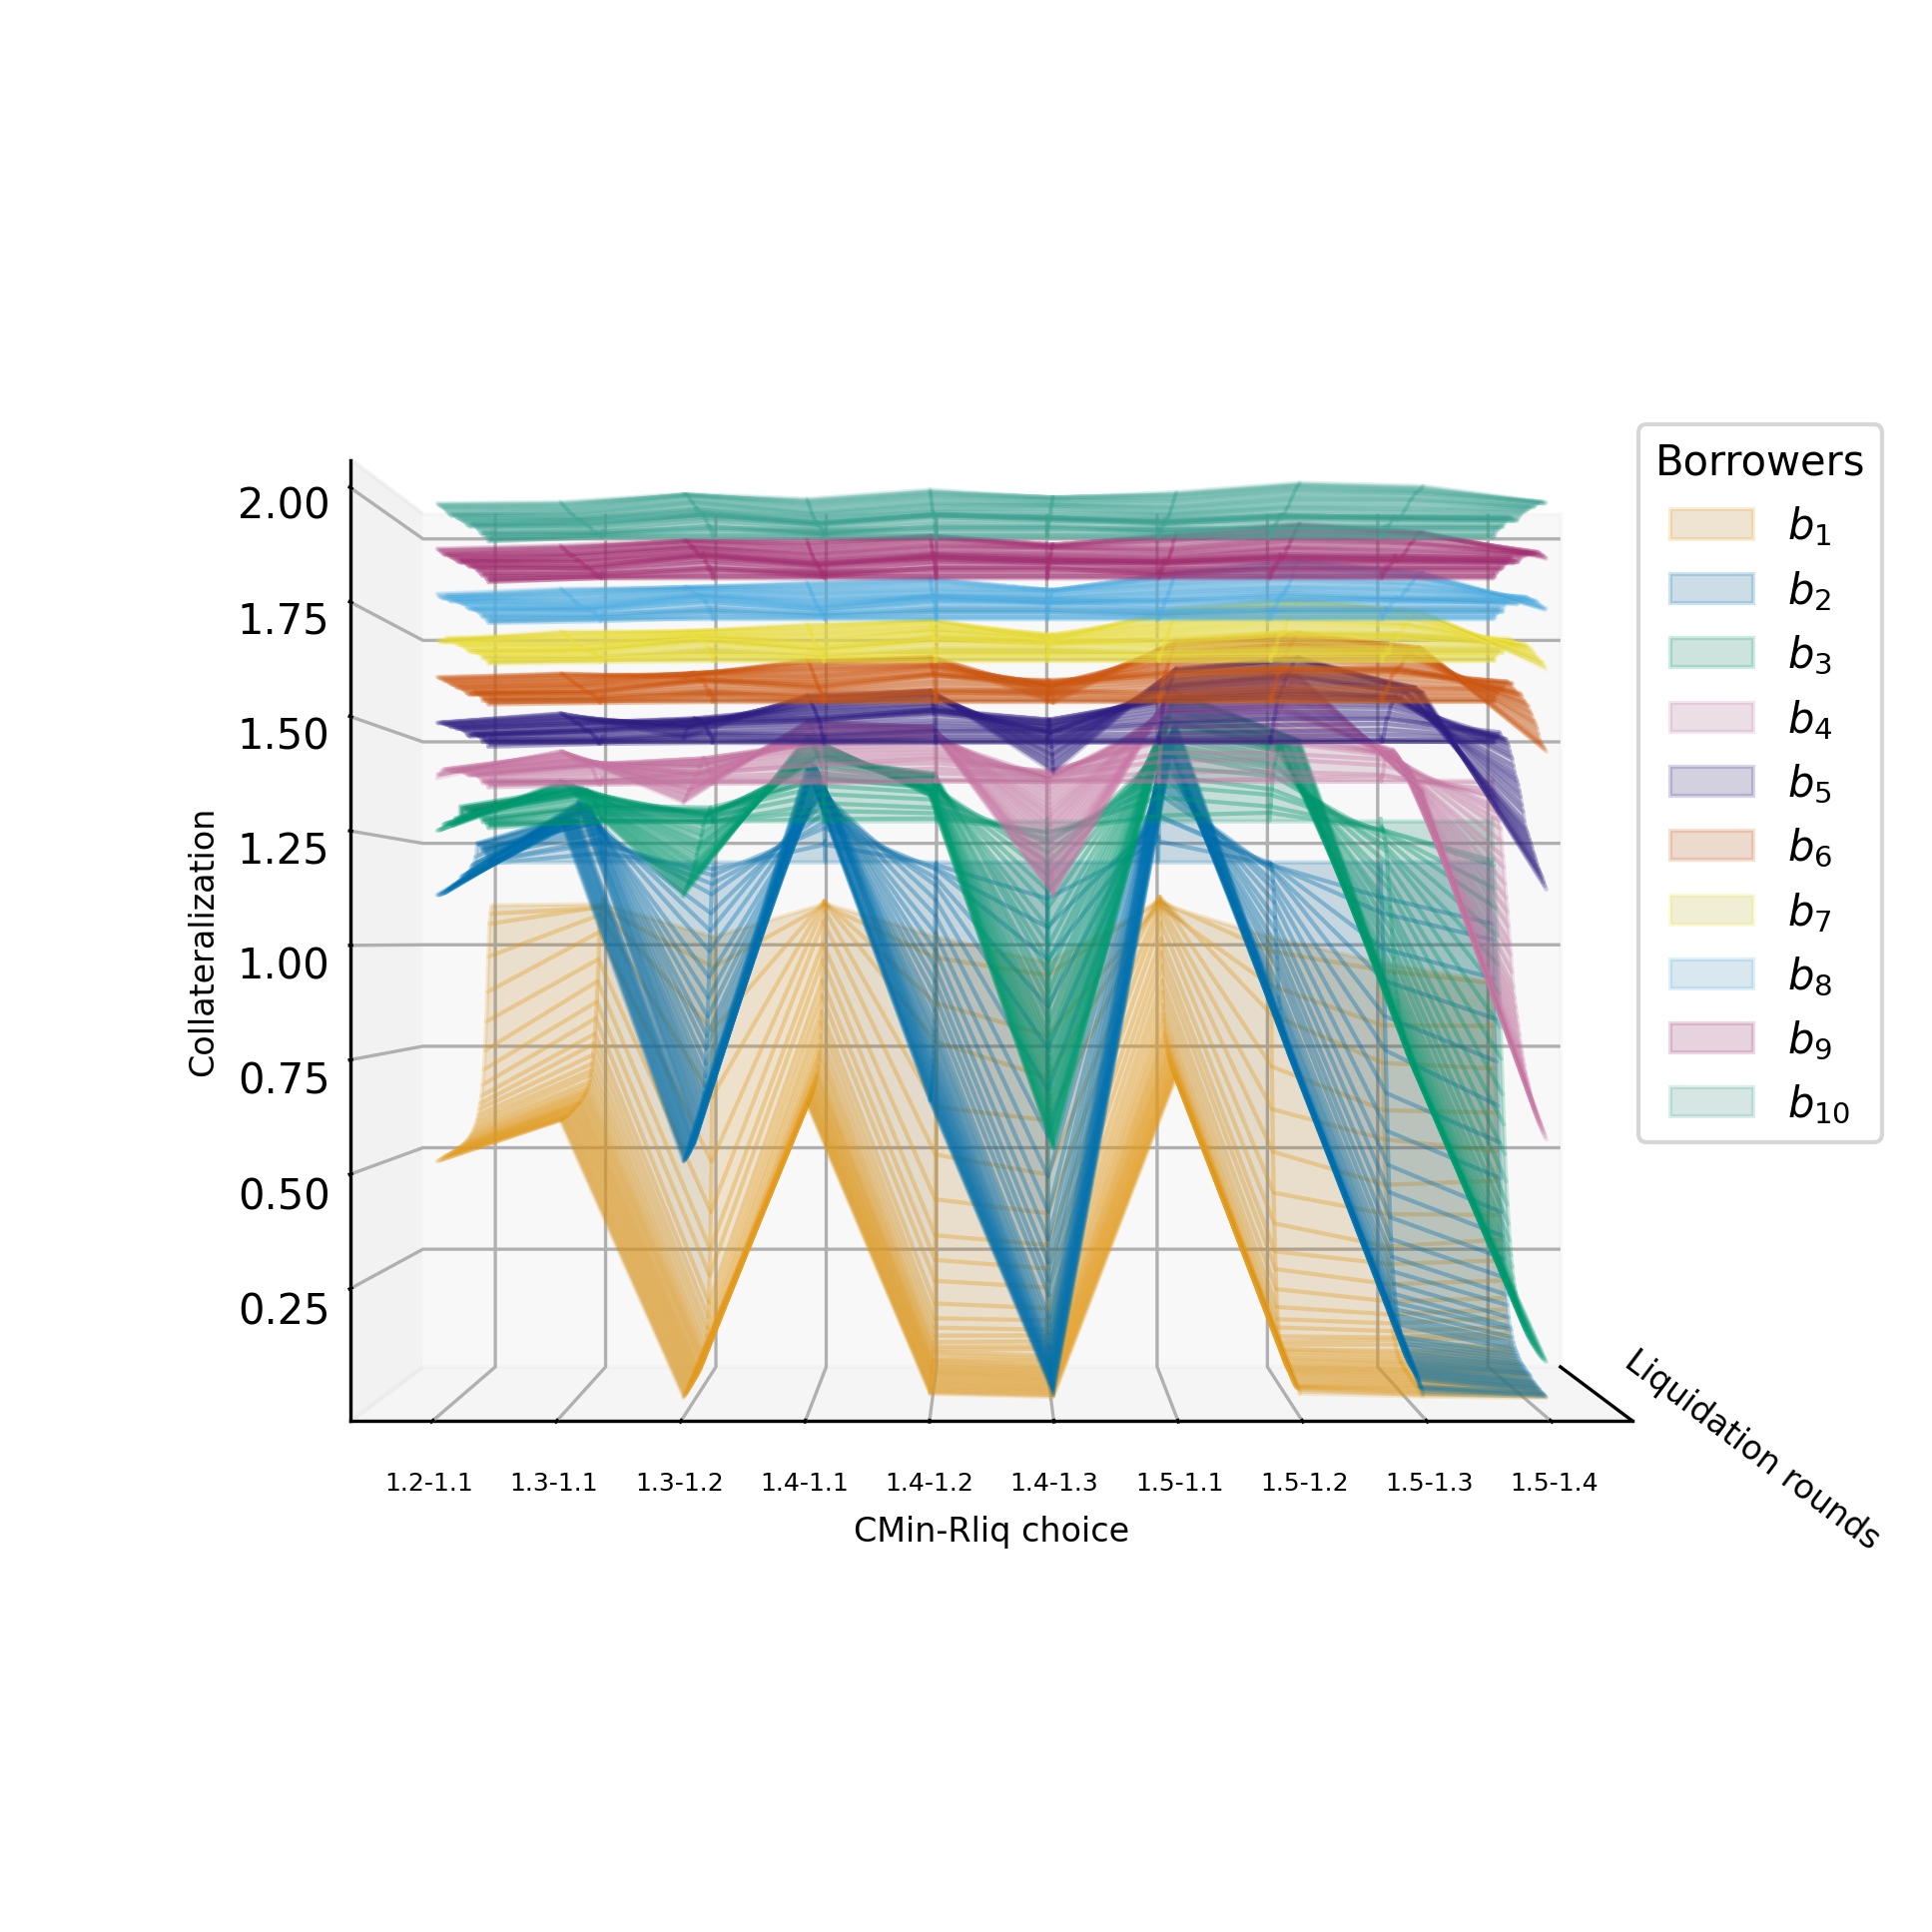}
    \caption{Scenario: eth-wbtc.}
    \label{fig:s-eth-wbtc-cmin-rliq-ag_1_10}
  \end{subfigure}
\end{figure}
\begin{figure} \ContinuedFloat
  \centering
  % \medskip
  \begin{subfigure}[H]{\textwidth}
    \centering
    \includegraphics[angle=90]{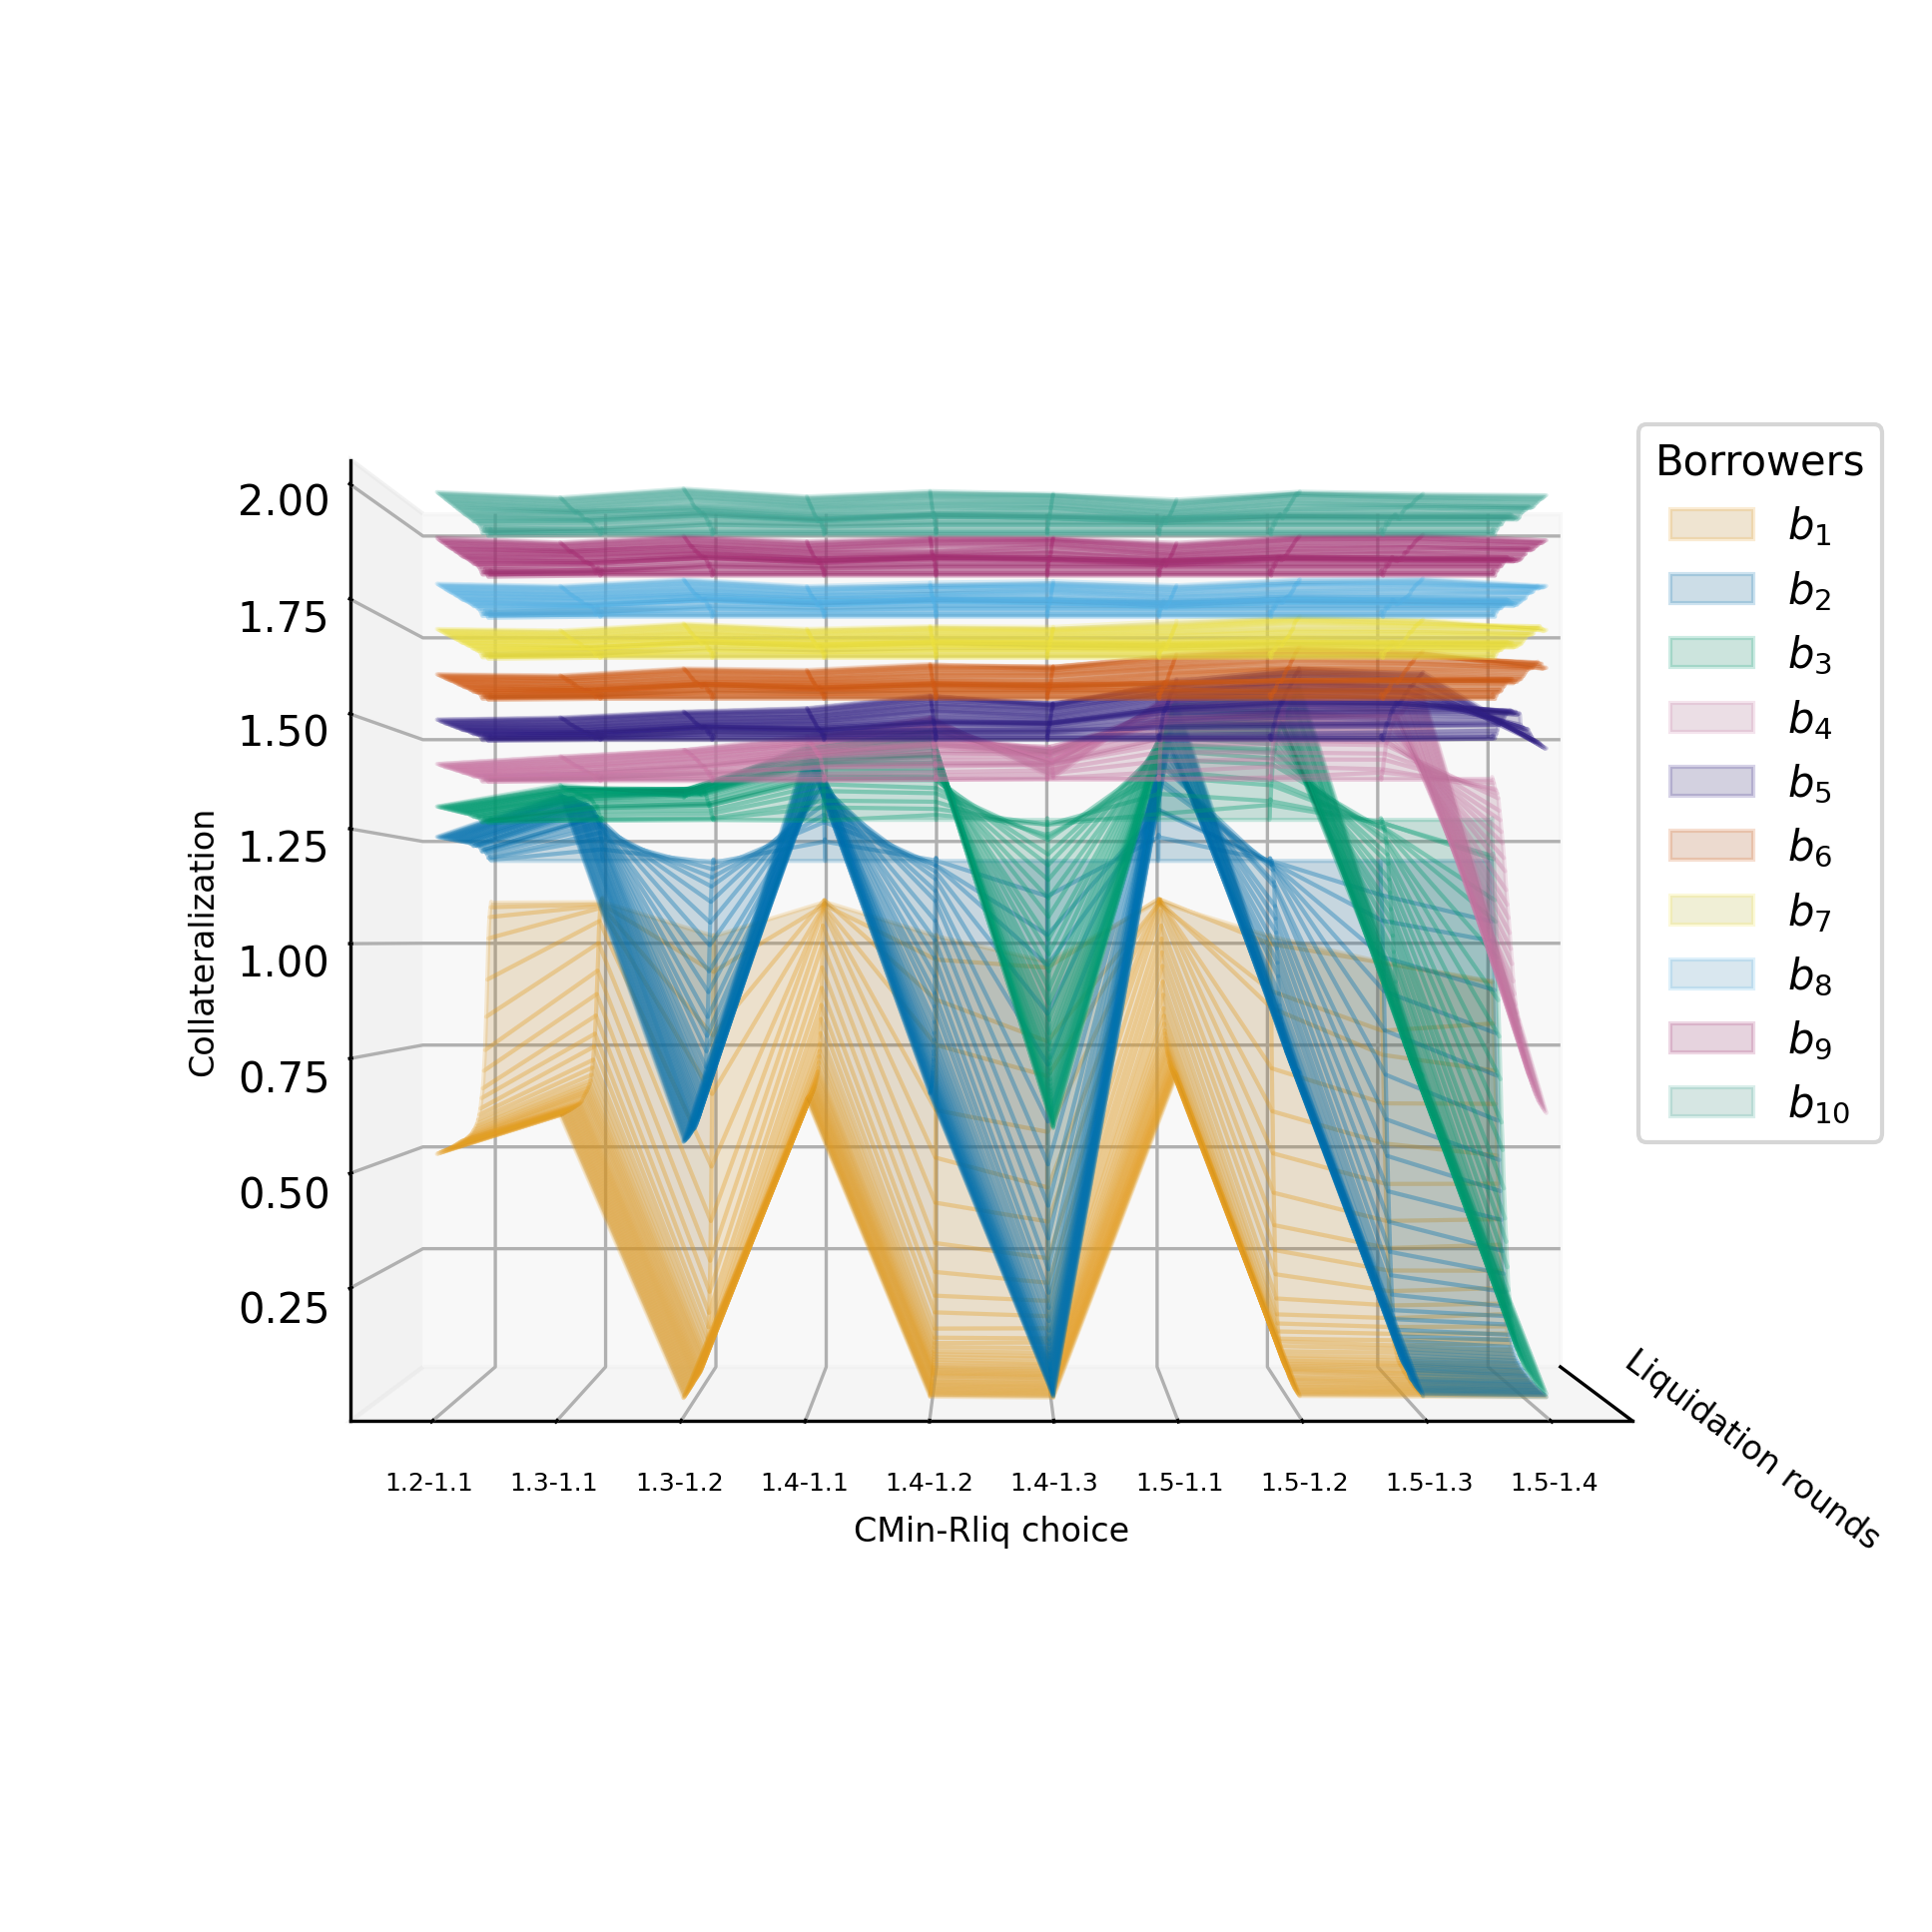}
    \caption{Scenario: eth-usdc.}
    \label{fig:s-eth-usdc-cmin-rliq-ag_1_10}
  \end{subfigure}
  % \medskip 
\end{figure}
\begin{figure} \ContinuedFloat
  \begin{subfigure}[H]{\textwidth}
    \centering
    \includegraphics[angle=90]{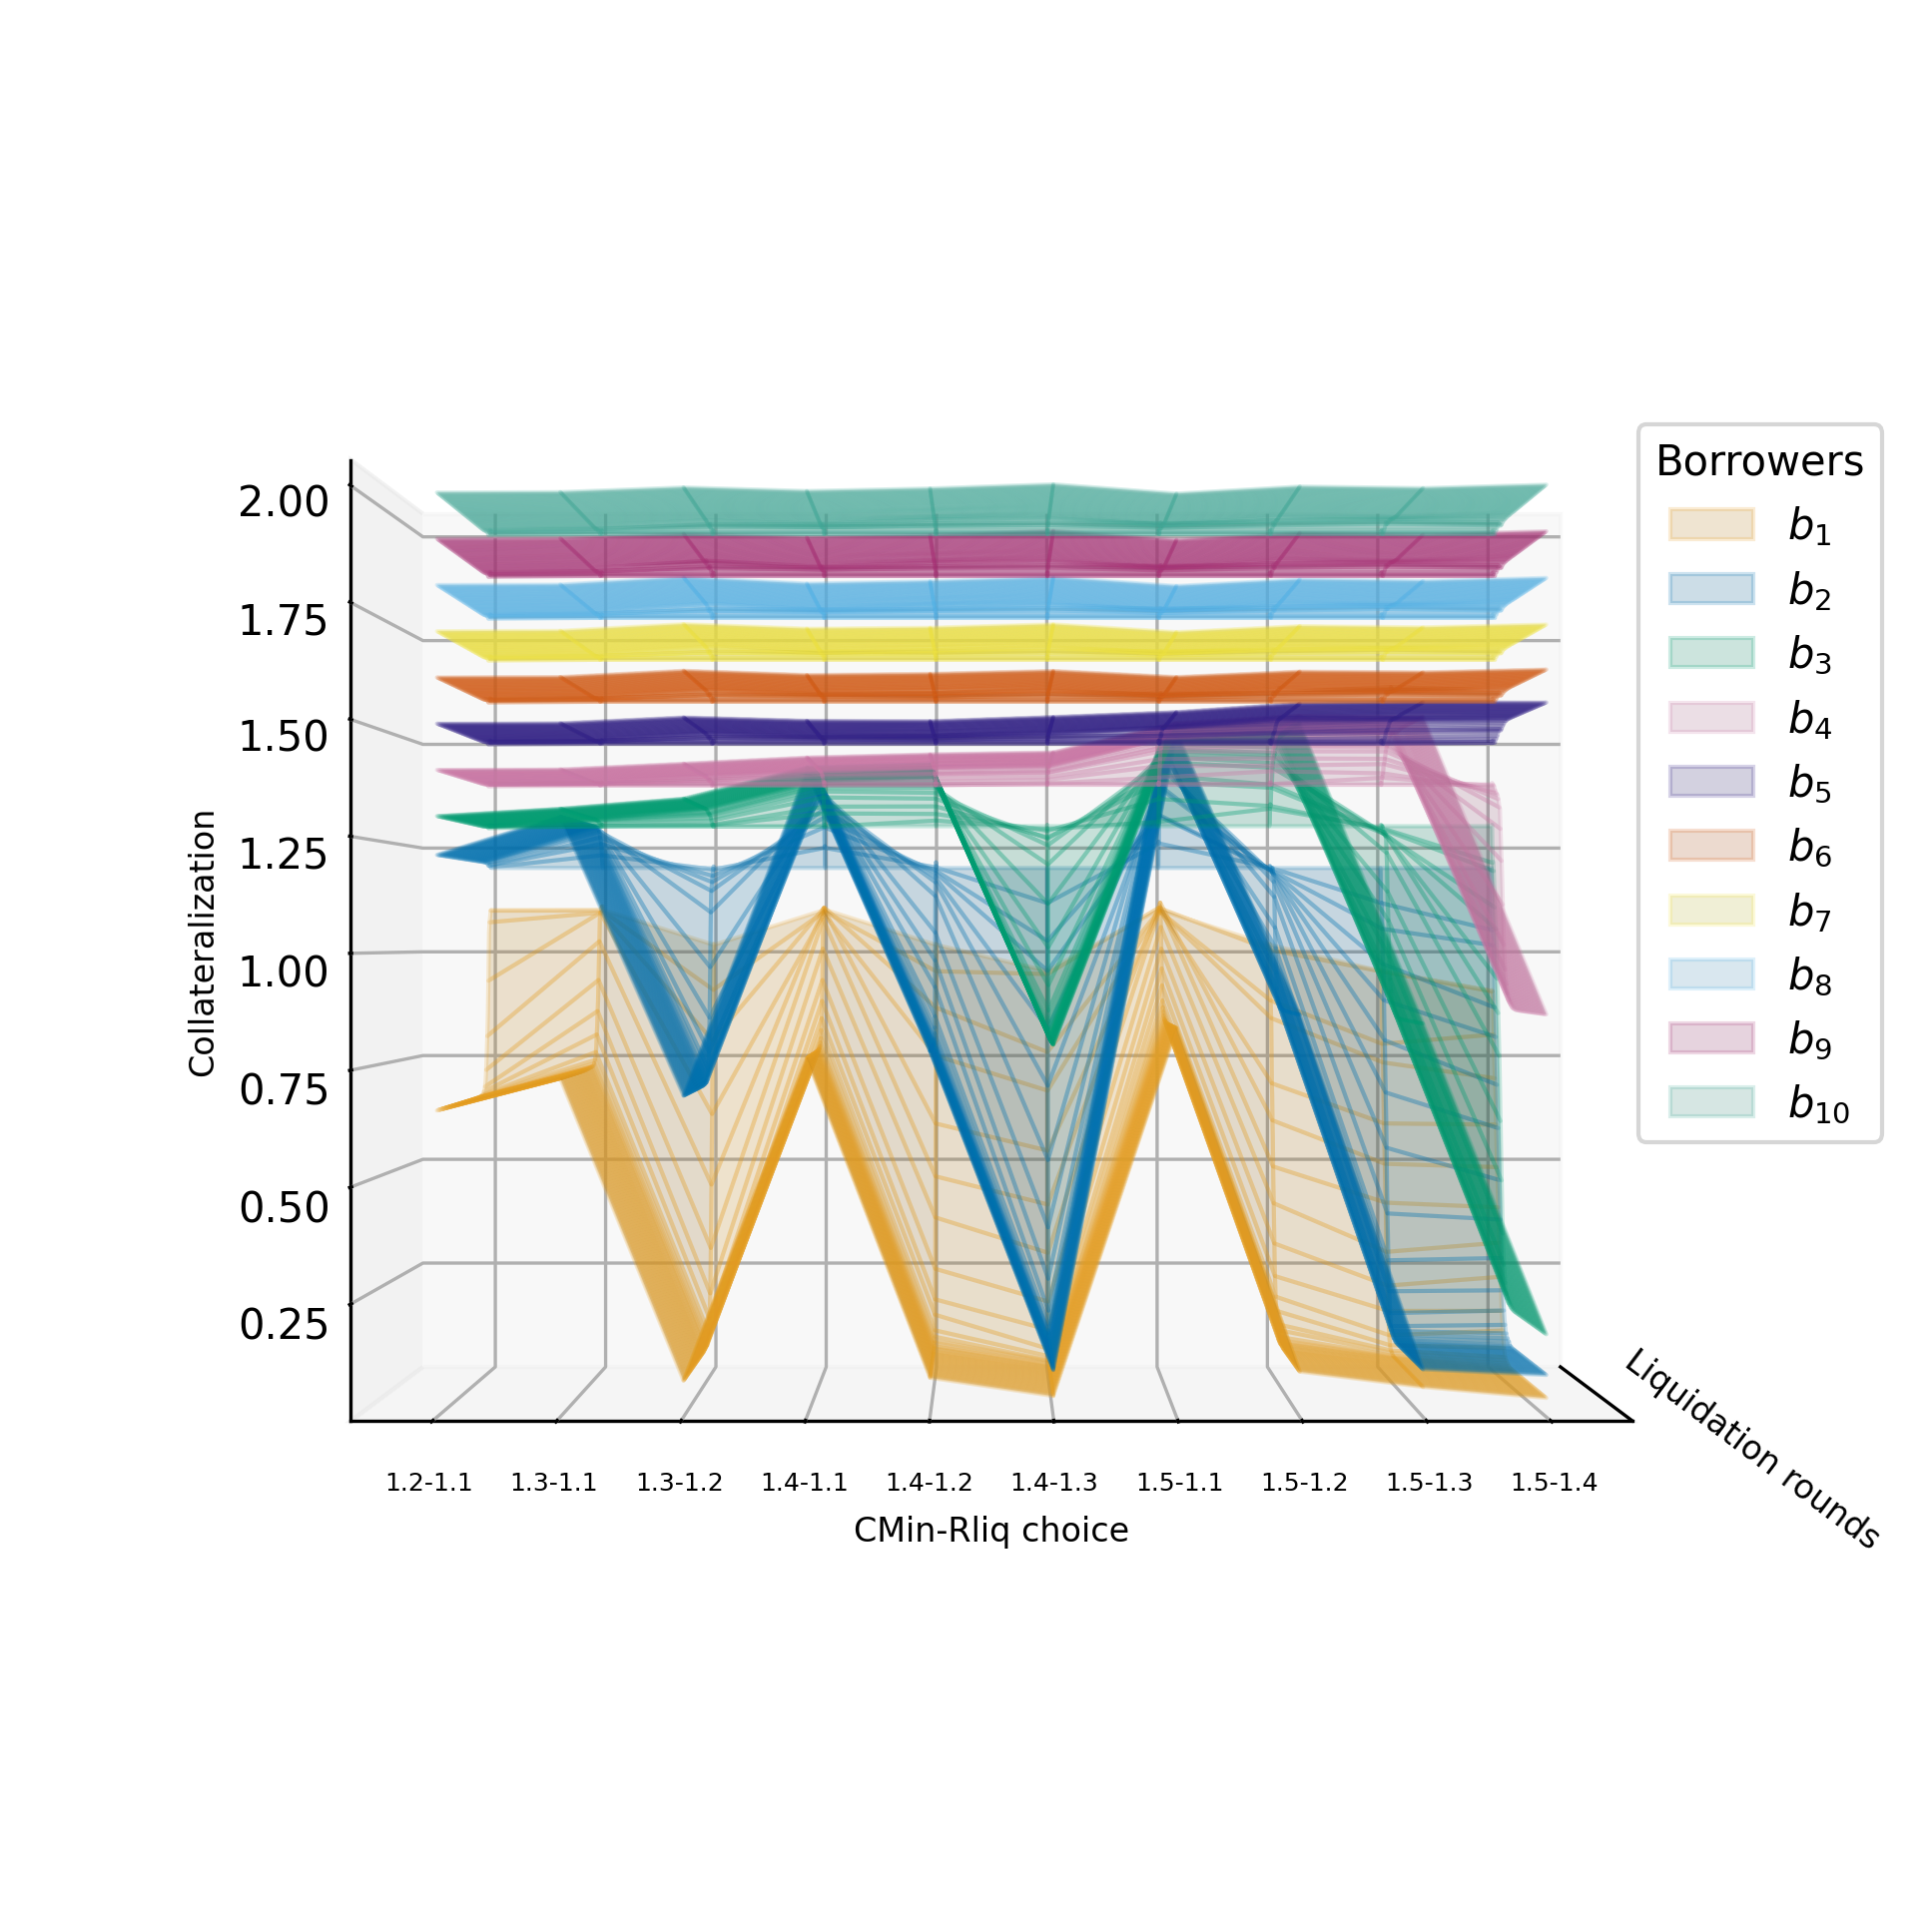}
    \caption{Scenario: usdc-wbtc.}
    \label{fig:s-usdc-wbtc-cmin-rliq-ag_1_10}
  \end{subfigure}
  \caption{Per-borrower collateralization in the three prices scenarios, with varying liquidation rounds and \texttt{CMin-rliq} choices.}
  \label{fig:3d-all}
\end{figure}

\clearpage

%\section{Lending pools simulation}
%
%\SecSubSec{Full running example}
%
%\begin{mdframed}[style=codeframe-style,
%                 innerbottommargin=\MListFrm\baselineskip]
%  \lstinputlisting[
%  %consecutivenumbers=false,  
%  style=maude-file-style,
%  language=maude,
%  caption={\texttt{search.maude} - Full running example representing the configurations in \Cref{tab:run-ex}},  
%  label=lst:search-run-ex-full,
%  ]{../model/results/search.maude}
%\end{mdframed}
%
